# Supplementary material for: Score-Based Generative Modeling with Critically-Damped Langevin Diffusion
Source: arXiv:2112.07068 source file (2022-03-25)
Supplement: Supplementary file 1 [file variance_reduction.tex]

\section{Variance Reduction} \label{app:variance_reduction}
\subsection{Control Variate}
Recall the simplified maximum likelihood objective~(\Cref{eq_app:simplified_maximum_likelihood_objective}):
\begin{align}
    \E_{t \sim \gU[0, 1], \varepsilon \sim \gN(\bm{0}, \mI_{2d}), \rvu = \vmu_t + \mL_t \varepsilon} \left[ \norm{\nabla_\rvz \log p_{0t}(\rvu \mid \rvu_0) - \nabla_\rvz \log q_{0t}(\rvu)}_2^2 \right].
\end{align}
The idea of the control variate is to add and subtract the following term within the expectation
\begin{align}
    \norm{\nabla_\rvz \log p_{0t}(\rvu \mid \rvu_0)}_2^2 - 2 \left[\nabla_\rvz \log p_{0t}(\rvu \mid \rvu_0)\right]^\top \nabla_\rvz \log q_{t}(\vmu_t).
\end{align}
In practice, we use the following control variates
\begin{align}
    C_{\mathrm{ML}}(t) &= - 2 \ell_t^2 \varepsilon_{d:2d}^\top \alpha_\vtheta(\vmu_t, t) + \ell_t^2 \norm{\varepsilon_{d:2d}}_2^2, \\
    \E_{t \sim \gU[0, 1], \varepsilon \sim \gN(\bm{0}, \mI_{2d}), \rvu = \vmu_t + \mL_t \varepsilon}\left[C_{\mathrm{ML}}(t)\right]&= \E_{t \in [0, 1]} [\ell_t^2] D,
\end{align}
and
\begin{align}
    C_{\mathrm{FID}}(t) &= - 2 \varepsilon_{d:2d}^\top \alpha_\vtheta(\vmu_t, t) + \norm{\varepsilon_{d:2d}}_2^2, \\
    \E_{t \sim \gU[0, 1], \varepsilon \sim \gN(\bm{0}, \mI_{2d}), \rvu = \vmu_t + \mL_t \varepsilon}\left[C_{\mathrm{FID}}(t)\right] &= D.
\end{align}
The maximum likelihood objective functions with control variate is then given as
\begin{align}
    \gL_{\mathrm{ML}}^C &= \E_{t \sim \gU[0, 1], \varepsilon \sim \gN(\bm{0}, \mI_{2d}), \rvu = \vmu_t + \mL_t \varepsilon} \left[ \ell_t^2 \norm{\varepsilon_{d:2d} - \alpha_\vtheta(\rvu, t)}_2^2 -C_{\mathrm{ML}}(t) + C_{\mathrm{ML}}(t)\right] \\
    &=\E_{t \sim \gU[0, 1], \varepsilon \sim \gN(\bm{0}, \mI_{2d}), \rvu = \vmu_t + \mL_t \varepsilon} \left[\ell_t^2 \norm{\alpha_\vtheta(\rvu, t)}_2^2 - 2 \ell_t^2 \varepsilon_{d:2d}^\top \left[ \alpha_\vtheta (\rvu, t) - \alpha_\vtheta (\vmu_t, t)\right] + \ell_t^2 D\right].
\end{align}
In practice, we can simply drop the last term in the expectation as it is independent of $\vtheta$. The simplified objective function with control variate is given as
\begin{align}
    \gL_{\mathrm{FID}}^C &= \E_{t \sim \gU[0, 1], \varepsilon \sim \gN(\bm{0}, \mI_{2d}), \rvu = \vmu_t + \mL_t \varepsilon} \left[\norm{\varepsilon_{d:2d} - \alpha_\vtheta(\rvu, t)}_2^2 -C_{\mathrm{FID}}(t) + C_{\mathrm{FID}}(t)\right] \\
    &=\E_{t \sim \gU[0, 1], \varepsilon \sim \gN(\bm{0}, \mI_{2d}), \rvu = \vmu_t + \mL_t \varepsilon} \left[\norm{\alpha_\vtheta(\rvu, t)}_2^2 - 2 \varepsilon_{d:2d}^\top \left[ \alpha_\vtheta (\rvu, t) - \alpha_\vtheta (\vmu_t, t)\right] + D\right],
\end{align}
where we again can drop the last term.
\subsection{Importance Sampling}
We follow the importance sampling strategy from~\citet{vahdat2021score}. In particular, we assume that
\begin{align}
    p_0 &= \gN(\bm{0}, \overline \mSigma_t), \\
    \overline \mSigma_0 &= \begin{pmatrix} 1 & 0 \\ 0 & \gamma M \end{pmatrix} \otimes \mI_d, \quad \gamma \in [0, 1].
\end{align}
The diffused distribution at time $t$ is then Gaussian with mean and covariance following the following initial value problems
\begin{align} \label{eq:mean_ode_variance_reduction}
    \frac{d\vmu_t}{dt} = \mF \vmu_t, \\
    \vmu_0 = \bm{0}, \label{eq:mean_initial_condition_variance_reduction}
\end{align}
and
\begin{align} \label{eq:variance_ode_variance_reduction}
    \frac{d\overline\mSigma_t}{dt} &= \mF \mSigma_t + \left[ \mF \mSigma_t \right]^\top + \mL \mL^\top, \\
    \overline \mSigma_0 &= \overline \mSigma_0. \label{eq:variance_initial_condition_variance_reduction}
\end{align}
It is easy to see that $\vmu_t = \bm{0}$. Furthermore, we have
\begin{align}
    \overline \mSigma_t &= \mK \otimes \mI_d, \\
    \mK &= \begin{pmatrix} e^{4\beta\Gamma^{-1} t} + 4 \beta^2 \Gamma^{-2} t^2 (\gamma - 1) & (\gamma - 1) (\beta t - 2 \beta^2 \Gamma^{-1} t^2) \\ (\gamma - 1) (\beta t - 2 \beta^2 \Gamma^{-1} t^2) &\frac{\Gamma^2}{4} e^{4\beta\Gamma^{-1} t}  + (\gamma - 1) (\Gamma^2 / 4 + \beta^2 t^2 - \Gamma \beta t)\end{pmatrix} e^{-4\beta\Gamma^{-1} t}.
\end{align}
Note that for $\gamma = 1$, we have $\overline \Sigma_t = \overline \Sigma_0$. We will need the inverse of $\overline \mSigma_t$ later, so let us compute it now:
\begin{align}
    \overline \mSigma_t^{-1} &= (\mK \otimes \mI_d)^{-1} \\
    &= \mK^{-1} \otimes \mI_d, \\
    \mK^{-1} &= \tfrac{1}{\emK_{11} \emK_{2} - \emK_{12}^2}\begin{pmatrix} \emK_{22} & - \emK_{12} \\ -\emK_{12} &\emK_{22} \end{pmatrix}.
\end{align}

The score $\nabla_\rvz \log p_t(\rvu)$ can then be computed as
\begin{align}
    \nabla_\rvz \log p_t(\rvu) &= -\left[\overline \mSigma_t^{-1} \rvu\right]_{d:2d} \\
    &= -\left[\overline \mSigma_t^{-1}  (\vmu_t + \overline \mL_t \varepsilon) \right]_{d:2d} \\
    &= -\left[\overline \mSigma_t^{-1}  \vmu_t + \overline \mL_t^{-\top} \varepsilon \right]_{d:2d}, \label{eq_app:decomposed_score}
\end{align}
where $\overline \mL_t \overline \mL_t^\top$ is the Cholesky factorization of $\mSigma_t$. We will now derive four importance sampling distributions: one with and one without the control variate for each of the two weightings (ML and FID). As an important ingredient, we will be using~\Cref{eq_app:decomposed_score} as well as~\Cref{eq:gradient_gaussian_transition_kernel}. 
\subsubsection{ML without Control Variate}
We have
\begin{align}
    \mathrm{ML}(t) &= \E \left[ \norm{\nabla_\rvz \log p_{0t}(\rvu \mid \rvu_0) - \nabla_\rvz \log q_{t}(\rvu)}_2^2 \right] \\
    &= \E \left[\norm{\left[\overline \mSigma_t^{-1} \vmu_t\right]_{d:2d} + (\overline \ell_t - \ell_t) \varepsilon_{d:2d}}_2^2\right] \\
    &= \E \left[\norm{\left[\overline \mSigma_t^{-1} \vmu_t\right]_{d:2d}}_2^2 \right] + (\overline \ell_t - \ell_t)^2 d,
\end{align}
where unidentified expectations are with respect to $\varepsilon \sim \gN(\bm{0}, \mI_{2d})$ and $\rvu = \vmu_t + \mL_t \varepsilon$. It is now left to compute $\E \left[\norm{\left[\overline \mSigma_t^{-1} \vmu_t\right]_{d:2d}}_2^2 \right]$:
\begin{align}
    \E \left[\norm{\left[\overline \mSigma_t^{-1} \vmu_t\right]_{d:2d}}_2^2 \right] &= \E \left[\norm{\emK^{-1}_{21} \left[\vmu_t\right]_{0:d} + \emK^{-1}_{22} \left[\vmu_t\right]_{d:2d}}_2^2 \right] \\
    &= \left(\emK_{11} \emK_{2} - \emK_{12}^2\right)^{-2} \E\left[\norm{\emK_{11} \left[\vmu_t\right]_{2:2d} -\emK_{12} \left[\vmu_t\right]_{0:d}}_2^2\right].
\end{align}
Plugging in the definition of the mean~(\Cref{eq:mean_solution}), we have
\begingroup\makeatletter\def\f@size{8}\check@mathfonts
\begin{align}
    \E \left[\norm{\left[\overline \mSigma_t^{-1} \vmu_t\right]_{d:2d}}_2^2 \right] &= \iota(t) \E\left[\norm{\emK_{11} \left[- \beta t \rvx(0) - 2 \beta t \Gamma^{-1} \rvz(0) + \rvz(0)\right] -\emK_{12} \left[2 \beta \Gamma^{-1} t \rvx(0) + 4 \beta t \Gamma^{-2} \rvz(0) + \rvx(0)\right]}_2^2\right] \\
    &= \iota(t) \E\left[\norm{\rvx(0) \left[-\beta t \emK_{11} - 2 \beta t \Gamma^{-1} \emK_{12} - \emK_{12} \right] + \rvz(0) \left[-2\beta t \Gamma^{-1} \emK_{11} + \emK_{11} - 4 \beta t \Gamma^{-2} \emK_{12} \right]}_2^2\right] \\
    &= \iota(t) d \left[-\beta t \emK_{11} - 2 \beta t \Gamma^{-1} \emK_{12} - \emK_{12} \right]^2 + \iota d \gamma M \left[-2\beta t \Gamma^{-1} \emK_{11} + \emK_{11} - 4 \beta t \Gamma^{-2} \emK_{12} \right]^2_2,
\end{align}
\endgroup
where $\iota(t) \coloneqq \left(\emK_{11} \emK_{2} - \emK_{12}^2\right)^{-2} e^{-4 \beta \Gamma^{-1} t}$.
\subsubsection{FID without Control Variate}
\begin{align}
    \mathrm{FID}(t) &= \ell_t^{-2} \E \left[ \norm{\nabla_\rvz \log p_{0t}(\rvu \mid \rvu_0) - \nabla_\rvz \log q_{t}(\rvu)}_2^2 \right] \\
    &= \E \left[\norm{\ell_t^{-1} \left[\overline \mSigma_t^{-1} \vmu_t\right]_{d:2d} + (\ell_t^{-1} \overline \ell_t - 1) \varepsilon_{d:2d}}_2^2\right] \\
    &= \ell_t^{-1}\E \left[\norm{\left[\overline \mSigma_t^{-1} \vmu_t\right]_{d:2d}}_2^2 \right] + (\ell_t^{-1} \overline \ell_t - 1)^2 d.
\end{align}
\subsubsection{ML with Control Variate}
\begin{align}
    \mathrm{MLC}(t) &= \E \left[ \norm{\nabla_\rvz \log q_{t}(\rvu)}_2^2 - 2 \left[\nabla_\rvz \log p_{0t}(\rvu \mid \rvu_0)\right]^\top \left[\nabla_\rvz \log q_{t}(\rvu) - \nabla_\rvz \log q_{t}(\vmu_t)\right] \right] \\
    &= \E \left[\norm{\left[\overline \mSigma_t^{-1} \vmu_t\right]_{d:2d}}_2^2 \right] + \overline \ell_t^2 d - 2 \E\left[\left[-\ell_t \varepsilon_{d:2d}\right]^\top \left[- \overline \ell_t \varepsilon_{d:2d} \right] \right] \\
    &= \E \left[\norm{\left[\overline \mSigma_t^{-1} \vmu_t\right]_{d:2d}}_2^2 \right] + \left(\overline \ell_t^2 - 2 \ell_t \overline \ell_t \right)d.
\end{align}
\subsubsection{FID with Control Variate}
\begin{align}
    \mathrm{FIDC}(t) &= \ell_t^{-2} \E \left[ \norm{\nabla_\rvz \log q_{t}(\rvu)}_2^2 - 2 \left[\nabla_\rvz \log p_{0t}(\rvu \mid \rvu_0)\right]^\top \left[\nabla_\rvz \log q_{t}(\rvu) - \nabla_\rvz \log q_{t}(\vmu_t)\right] \right] \\
    &= \ell_t^{-1} \E \left[\norm{\left[\overline \mSigma_t^{-1} \vmu_t\right]_{d:2d}}_2^2 \right] + (\ell_t^{-2} \overline \ell_t^2 - 2 \ell_t^{-1} \overline \ell_t) d.
\end{align}
\subsection{Approximate and Mixed Importance Sampling}
